# Supplementary material for: How robust accuracy suffers from certified training with convex relaxations
Source: arXiv:2306.06995 source file (2023-06-12)
Supplement: Supplementary file 1 [file aux_lemmas.tex]

\subsection{Proof of~\Cref{lemma:robust_risk}}
\robustrisk*
\begin{proof}
Without loss of generality, we assume that  $\psig >0$, and since $a$ and $b$ are not trainable parameters, we must have $a>0$ and $b<0$ to solve the classification problem. The robust error is then equal to
\begin{align*}
\rrisk(\theta)  &\defn  \prob_{(x, y)}\left[\exists z \in \BB_\epsilon(x) : y \neq \sgn\left(\nn(z)\right)\right] \\
&= \frac{1}{2} \left(\prob_{x}\left[a\relu{\theta^\top x}  + b< 0 \mid y=1 \right] + \prob_{x}\left[a\relu{\theta^\top x}  + b> 0 \mid y=-1\right]\right).
\end{align*}
Further, we can remove the \(\relu{\cdot}\) using the fact that \(\frac{b}{a}<0\):
\begin{align*}
\rrisk(\theta)  &= \frac{1}{2} \left(\prob_{x}\left[\{x: \theta^\top x + \frac{b}{a}< 0 \lor \theta^\top x < 0 \} \mid y=1 \right] + \prob_{x}\left[\{x: \theta^\top x  + \frac{b}{a}> 0 \land \theta^\top x  >0 \}\mid y=-1\right]\right) \\
&=\frac{1}{2} \left(\prob_{x}\left[ \theta^\top x + \frac{b}{a}< 0 \mid y=1 \right] + \prob_{x}\left[\ \theta^\top x  + \frac{b}{a}> 0 \mid y=-1\right]\right)\\
   &= \frac{1}{2}\left(\prob_{x}\left[ \sum_{i=2}^\di x_i \theta_i  < -\psig(\margin -\epsilon)-\frac{b}{a}\right] + \prob_{x}\left[ \sum_{i=2}^\di x_i \theta_i  > \psig(\margin -\epsilon)-\frac{b}{a}\right] \right).
   \end{align*}
   Recall now that for the linearly separable distribution we have \(\sum_{i=2}^\di x_i \theta_i \sim \gauss\left(0,\stdsig^2\norm{\pnoise}^2\right) \). Therefore, we can replace the probabilities with the standard normal CDF \(\Phi\):
   \begin{align*}
   \rrisk(\theta) &=  \frac{1}{2}\left (  \gausscdf \left(-\frac{(\margin-\epsilon)\psig} {\stdsig\norm{\pnoise}_2} - \frac{b}{a\stdsig\norm{\pnoise}_2}\right) + \gausscdf \left(-\frac{(\margin-\epsilon)\psig} {\stdsig\norm{\pnoise}_2} +\frac{b}{a\stdsig\norm{\pnoise}_2}\right) \right).
\end{align*}
Hence $\rrisk(\theta)$ is monotonically decreasing in $\theta_1$ and the statement follows.
\end{proof}

 \subsection{Proof of~\Cref{lemma:advgrad}}
The basic idea behind adversarial training is to update the network parameters according to the following rule:
\begin{align*}
	\theta \leftarrow \theta - \frac{\eta}{|D|} \sum_{(x,y) \in D} \nabla_\theta \max_{x+\delta \in \BB_{\epsilon}(x)} L(\nn(x + \delta),y).
\end{align*} 
This is usually done by applying some first-order approximation to the maximisation problem.  However, for our simplified network, we can analytically compute the gradient.
First of all, note that when \(L\) is the binary cross-entropy loss function, we can rewrite the maximisation problem as
\begin{equation}
\begin{aligned}
 \underset{x+\delta \in \BB_{\epsilon}(x)}{\operatorname{max}} L(\nn(x + \delta),y)
 = L \left(\sgn(y) \overbrace{\underset{x+\delta \in \BB_{\epsilon}(x)}{\operatorname{min}} \sgn(y) \nn(x+\delta)}^{\defn \advobj(x,y)},\;y \right).
\end{aligned}
\end{equation}
In particular, if \(\advobj\) is strictly positive, then no adversarial example exists that fools the network.% Further, note that this  formulation is closely related to the objective considered in \Cref{apx:certified_training} for the convex outer adversarial polytope. This will be useful when comparing \wong and \madry gradients.
 Below we provide the gradient of the adversarial training objective w.r.t. the network parameters \(\theta\).

\begin{proof}
Given a data point $x$ with known label $y \in \{-1,1\}$, when \(L\) is the binary cross-entropy loss function we have
\begin{equation*}
\begin{aligned}
 \underset{x+\delta \in \BB_{\epsilon}(x)}{\operatorname{max}} L(\nn(x + \delta),y)
 = L \left(\sgn(y) \underset{x+\delta \in \BB_{\epsilon}(x)}{\operatorname{min}} \sgn(y) \nn(x+\delta),\;y \right).
\end{aligned}
\end{equation*}
For our simplified network, we can analytically compute a closed-form solution to the minimisation problem
\begin{equation*}\label{eq:exact_j}
\begin{aligned}
    \advobj &\defn \underset{x+\delta \in \BB_\epsilon(x)}{\operatorname{min}} \sgn(y) \left(\bias + a\relu{\theta^\top (x+\delta)}\right) \\&=  \begin{cases} 
 \sgn(y) \left(\bias + a  \operatorname{max}(0,\plb) \right)& \; \text{if} \; \; a\sgn(y) > 0\\
 \sgn(y) \left(\bias + a \operatorname{max}(0,\pub) \right)& \; \text{if} \; \; a\sgn(y) < 0\\
   \end{cases} \\ \\ &=    \begin{cases} 
 \sgn(y) \left(\bias + a \operatorname{max}(0,\plb) \right)& \; \text{if} \; \; \ a\sgn(y) > 0\\
 \sgn(y) \left(\bias + a \operatorname{max}(0,\pub) \right)& \; \text{if} \; \; \ a\sgn(y) < 0,
   \end{cases} 
  \end{aligned}
\end{equation*}
where $\plb = \theta^\top x - \epsilon |\psig|$ and $\pub = \theta^\top x + \epsilon |\psig|$ are respectively lower and upper bounds on the pre-activations.
Thus, we can compute the gradients for adversarial training w.r.t the signal parameter
\begin{equation*}
\begin{aligned}
\frac{\partial}{\partial \psig} \advobj =  \begin{cases} 
 \sgn(y)a(\xsig - \epsilon \sgn(\psig))\indicator{ \plb> 0 }& \; \text{if} \; \; a\sgn(y) > 0\\
 \sgn(y) a(\xsig + \epsilon \sgn(\psig)) \indicator{ \pub > 0 }& \; \text{if} \; \; a\sgn(y) < 0,
   \end{cases} 
  \end{aligned}
\end{equation*}
and applying the chain rule, we have
\begin{align*}
    &\frac{\partial}{\partial \theta_{1}} \loss \left(\sgn(y)\advobj, y\right)\\ &= \frac{\partial}{\partial \advobj} \loss\left(\sgn(y)\advobj, y\right) \cdot  \frac{\partial}{\partial \theta_{1}} \advobj \\&=  \sgn(y)\left[\sigmoid{\sgn(y)\advobj }- \indicator{ y=1 } \right] \cdot \frac{\partial}{\partial \theta_{1}}\advobj\\
    &=   -\sgn(y)\sigmoid{-\advobj}  \begin{cases} 
a(x_1-\epsilon \sgn(\psig))\indicator{ \plb > 0 }& \; \text{if} \; \; a\sgn(y) > 0\\
 a (x_1+\epsilon \sgn(\psig))\indicator{ \pub> 0 }& \; \text{if} \; \; a\sgn(y) < 0, 
   \end{cases} 
\end{align*}
where in the last equality, we use a known property of the sigmoid function, \(\sigmoid{x} = 1-\sigmoid{-x}\). 
\end{proof}

\subsection{Certified training~(\wong)}
\label{apx:certified_training}
We now formulate the convex outer adversarial polytope~(\wong)~\citep{wong_provable_2018} for  adversaries that concentrate all their budget along the signal direction in the input. 



\paragraph{Network architecture} For the sake of clarity, we consider a 2-layers feed-forward ReLU network. However, our formulation can easily be extended to multiple layers. We define \(\nn(x):\RR^\di \to \RR^2\) as
\begin{equation}
\label{eq:lp_one_layer_net}
    x   \overset{x+\pert}{\longrightarrow} \hidden_1  \overset{\weight_1 \hidden_1+ b_1}{\longrightarrow} \hat{\hidden}_2 \overset{\relu{\cdot}}{\longrightarrow} \hidden_2 \overset{\weight_2 \hidden_2 + \bias_2}{\longrightarrow} \hat{\hidden}_3, 
\end{equation}
where  \(x \in \RR^{\di}\), \( \hidden_1 \in \BB_\epsilon(x) \), \(W_1\) and \(W_2\) are linear operators, and \(\theta=\{W_i,b_i\}_{i=1,2}\) is the set of network parameters. \newline \newline We define the adversarial polytope $\advpol(x)$ as the set of all final-layer activations attainable by perturbing $x$ with some $\xpert \in \BB_\epsilon(x)$:
\begin{align*}
    \advpol(x)= \{\nn(\xpert): \xpert \in \BB_\epsilon(x) \}.
\end{align*} 
The key idea behind \wong~\citep{wong_provable_2018} is to construct a convex outer bound to this adversarial polytope. Specifically, we relax the ReLU activations $\hidden_2= \relu{\hat{\hidden}_2}$ with their convex envelopes
\begin{align*}
      \hidden_2 \geq 0, \; \hidden_2 \geq \hat{\hidden}_2, \; (\pub-\plb)\hidden_2 \leq \pub \hat{\hidden}_2 - \pub \plb,
\end{align*}
where $\pub$ and $\plb$ are respectively the pre-activations \( \hat{\hidden}_2\) upper and lower bounds. We assume these bounds are known and provide a closed-form solution to compute them in
~\Cref{lemma:bounds}. Further, let $\advoutbound(x)$ be the outer bound to the adversarial polytope obtained from relaxing the ReLU constraints. Then, given a data point $x$ with known label $y$, we can formalise the problem of finding an adversarial example with a linear program as
\begin{equation}
\label{eq:adv_lp}
\underset{\hat{\hidden}_{3}}{\operatorname{min}}\; [\hat{\hidden}_{3}]_{y} - [\hat{\hidden}_{3}]_{\bar{y}} = c^\top \hat{\hidden}_3 \;\; \quad \text {s.t.} \;\; \hat{\hidden}_3 \in \advoutbound(x),
\end{equation}
where $\bar{y}$ is the binary negation of $y$. Note that if we solve this linear program and find that the objective is positive, then we know that no input perturbation within the threat model can misclassify the example. However, solving  the linear program in~\Cref{eq:adv_lp} for every example in the dataset is intractable. Therefore, we solve the dual formulation stated in the corollary below. Our derivation can be seen as an extension of the main results in~\citet{wong_provable_2018,erdemir_adversarial_2021}. 
\begin{restatable}{corollary}{dualLP}
\label{thm:signal_dual_LP}
The dual of the linear program  \eqref{eq:adv_lp} can be written as
\begin{align*}
\begin{array}{ll}
\underset{\alpha}{\max} & \certobj\left(x , \backnn (c,\alpha)\right) \\
\text{s.t.} & \; \alpha_j \in [0,1], \; \forall j,
\end{array}
\end{align*}
where $\certobj(x,\dualz_1,\dualz_2, \dualz_3)$ is equal to
\begin{align*}
     -\sum_{i=1}^{2} \dualz_{i+1}^{\top} \bias_{i}+\sum_{j \in \I} \plb_{ j} [\dualz_2]_j^+-\hat{\dualz}_1^{\top} x- \epsilon |[\hat{\dualz}_1]_1|,
\end{align*}
and $\backnn$ is a one-hidden layer neural network given by the equations
\begin{equation*}
    \begin{array}{ll}
& \dualz_{3}= -c \\
& \hat{\dualz_2} = \weight_2^\top\dualz_3\\
& [\dualz_{2}]_j=0, \;j \in \I^{-} \\
& [\dualz_2]_{ j}=\left[\hat{\dualz}_2\right]_{j}, \;j \in \I^{+} \\
&[\dualz_2]_{j} = \frac{\pub_j}{\pub_j-\plb_j}[\hat{\dualz}_2]_j^+ - \alpha_j[\hat{\dualz}_2]_j^- , \; j \in \I\\
& \hat{\dualz_1} = \weight_1^\top\dualz_2,
\end{array}
\end{equation*}
where $\I^-,\I^+$ and $\I$ denote the sets of activations  in the hidden layer where $\plb$ and $\pub$ are both negative, both positive or span zero, respectively. 
\end{restatable}
%Further, we take the feasible solution \( \alpha_j = \frac{\pub_j}{\pub_j-\plb_j}\), as proposed in~\citet{wong_provable_2018}. Hence, we can represent the
%dual problem  as a linear back propagation network, which provides a tractable
%solution for a lower bound of the primal objective.


 %\dualLP*
\begin{proof}
Consider a data point $x$ and let $\xpert = x + \delta$ be the adversarial perturbed data point. First, we explicit all the constraints for the linear program defined in \eqref{eq:adv_lp}:
\begin{equation*}
\begin{aligned}
&\underset{\hat{\hidden}_{3}}{\min}\; [\hat{\hidden}_{3}]_{y} - [\hat{\hidden}_{3}]_{\bar{y}} = c^\top \hat{\hidden}_3 \;, \quad \text { s.t. } \\
& x+\pert \in \BB_\epsilon(x) \\
& \hidden_1 = x+ \pert  \\
&\hat{\hidden}_{2}=\weight_{1} \hidden_{1}+\bias_{1} \\
&\hat{\hidden}_{3}=\weight_{2} \hidden_{2}+\bias_{2} \\
&[\hidden_2]_j=0,  \; \forall j \in \I^{-} \\
&[\hidden_2]_j= [\hat{\hidden}_2]_j , \; \forall j \in \I^{+}\\
& [\hidden_2]_j \geq 0, \;  \forall j \in \I\\
& [\hidden_2]_j \geq [\hat{\hidden}_2]_j, \;  \forall j \in \I\\ 
& \left(\left(\pub_j - \plb_j \right) [\hidden_2]_j\right. 
\left.-\pub_j [\hat{\hidden}_2]_j\right) \leq-\pub_j   \plb_j, \;  \forall j \in \I,
\end{aligned}
\end{equation*}
where  $\I^-, \I^+$  and $\I$  denote the sets of activations in the hidden layer where $\plb$ and $\pub$ are both negative, both positive or span zero, respectively. In order to compute the dual of this problem, we associate the following Lagrangian variables with each of the constraints:
\begin{equation*}
    \begin{aligned}
\hat{\hidden}_{2} &=\weight_{1} \hidden_{1}+\bias_{1} \Rightarrow \dualz_{2} \\
\hat{\hidden}_{3} &=\weight_{2} \hidden_{2}+\bias_{2} \Rightarrow \dualz_{3} \\
\hidden_{1}&= x+ \pert \Rightarrow \psi \\
-[\hidden_2]_j & \leq 0 \Rightarrow \mu_j, \;  \forall j \in \I \\
[\hat{\hidden}_2]_{j} -[\hidden_2]_j & \leq 0 \Rightarrow \tau_{j}, \;  \forall j \in \I \\
\left(\left(u_j -\plb_{j}\right) [\hidden_2]_j - \pub_j [\hat{\hidden}_2]_{j}\right) & \leq-\pub_j \plb_j \Rightarrow \lambda_{j}, \;  \forall j \in \I.
\end{aligned}
\end{equation*}
Note that we do not define explicit dual variables for $[\hidden_2]_j=0$ and $[\hidden_2]_j = [\hat{\hidden}_2]_j$  as we can easily eliminate them. We  write the Lagrangian as
\begin{equation*}
\begin{aligned}
\LL(\hidden, \hat{\hidden}, \dualz, \pert, \lambda, \tau, \mu, \psi)=&-\left(\weight_{1}^{\top} \dualz_{2}+\psi\right)^{\top} \hidden_{1}-\sum_{\substack{
j \in \I}}\left(\mu_{ j}+\tau_{ j}-\lambda_{ j}\left(\pub_{j}-\plb_{j}\right)+\left[\weight_{2}^{\top} \dualz_{3}\right]_{j}\right) [\hidden_2]_{j} \\
&+\sum_{\substack{j \in \I}}\left(\tau_{j}-\lambda_{ j} \pub_{ j}+[\dualz_2]_{ j}\right) [\hat{\hidden}_2]_{j}+\left(c+\dualz_{3}\right)^{\top} \hat{\hidden}_{3}-\sum_{i=1}^{2} \dualz_{i+1}^{\top} \bias_{i} \\
&+\sum_{\substack{j \in \I}} \lambda_{j} \pub_{j}\plb_{j}+\psi^{\top} x+\psi^{\top} \pert   
+ \sum_{j \in \I^-} [\hat{\hidden}_2]_j [\dualz_2]_j  \\
& + \sum_{j \in \I^+} [\hidden_2]_j \left([\dualz_2]_j - [\weight_2^\top \dualz_3]_j \right) \\
\text { s.t. } \xpert \in \BB_\epsilon(x),
\end{aligned}
\end{equation*}
and we take the infimum w.r.t. $\hidden,\hat{\hidden},\pert$
\begin{equation*}
    \begin{aligned}
\inf _{\hidden, \hat{\hidden}, \pert} \LL(\hidden, \hat{\hidden}, \dualz, \pert, \lambda, \tau, \mu, \psi)=&-\inf _{\hidden_2} \sum_{\substack{
j \in \I}}\left(\mu_{ j}+\tau_{ j}-\lambda_{ j}\left(\pub_{j}-\plb_{j}\right)+\left[W_{2}^{\top} \dualz_{3}\right]_{j}\right) [\hidden_2]_{j} \\
&+\inf _{\hat{\hidden}_2} \sum_{\substack{j \in \I}}\left(\tau_{j}-\lambda_{ j} u_{ j}+ [\dualz_2]_{ j} \right)  [\hat{\hidden}_2]_{ j}+\inf _{\hat{\hidden}_3}\left(c+\dualz_{3}\right)^{\top} \hidden_{3} -\sum_{i=1}^{2} \dualz_{i+1}^{\top} b_{i} \\
&+\sum_{\substack{
j \in \I}} \lambda_{j} \pub_{j} \plb_{j}+\psi^{\top} x+\inf _{ \xpert \in \BB_\epsilon(x)} \psi^{\top} \pert-\inf _{\hidden_{1}}\left(W_{1}^{\top} \dualz_{2}+\psi\right)^{\top} \hidden_{1} \\ &+ \inf _{\hat{\hidden}_{2}}\sum_{j \in \I^-} [\hat{\hidden}_2]_j [\dualz_2]_j  
 +\inf _{\hidden_{2}} \sum_{j \in \I^+} [\hidden_2]_j \left([\dualz_2]_j - [W_2^\top \dualz_3]_j \right).
\end{aligned}
\end{equation*}
Now, we can compute the infimum for the $\psi^\top \delta$ term:
\begin{equation*}
\inf _{ \xpert \in \BB_\epsilon(x)} \psi^{\top} \pert = \inf _{ \norm{\beta}_1\leq \epsilon} \psi_1  \cdot \beta = -\epsilon\cdot \norm{\psi_1}_1,
\end{equation*}
and since for all the other terms, the infimum of a linear function is $-\infty$, except in the special case when it is identically zero, the infimum of $\LL(\cdot)$ becomes
\begin{equation*}
\inf _{\hidden, \hat{\hidden}, \pert} \LL(.)= \begin{cases}-\sum_{i=1}^{2} \dualz_{i+1}^{\top} \bias_{i}+\sum_{j \in \I} \lambda_{ j} \pub_{j} \plb_{ j}+\psi^{\top} x- \epsilon \norm{\psi_1}_1& \text { if } \text { conditions } \\ -\infty & \text { else }\end{cases},
\end{equation*}
where the conditions to satisfy are
\begin{equation*}
\begin{aligned}
 & \dualz_{3}=-c\\
&W_{1}^{\top} \dualz_{2}=-\psi\\
&\left[\dualz_{2}\right]_{j}=0, j \in \I_{i}^{-}\\
&\left[\dualz_{2}\right]_{j}=\left[W_{2}^{\top} \dualz_{3}\right]_{j}, j \in \I_{i}^{+}\\
&\left.\begin{array}{ll}
\left(\pub_{j}-\plb_{j}\right) \lambda_{j}-\mu_{j}-\tau_{j} & =\left[W_{2}^{\top} \dualz_{3}\right]_{j} \\
{\left[\dualz_{2}\right]_{j}} & =\pub_{j} \lambda_{j}-\tau_{j}
\end{array}\right\} j \in \I\\
&\lambda, \tau, \mu \geq 0.
\end{aligned}
\end{equation*}
Thus, we can rewrite the dual problem as 
\begin{equation*}
\begin{aligned}
&\underset{\dualz, \psi, \lambda, \tau, \mu}{\max}-\sum_{i=1}^{2} \dualz_{i+1}^{\top} b_{i}+\sum_{j \in \I} \lambda_{j} \pub_{j} \plb_{j}+\psi^{\top} x-\epsilon \norm{\psi_{1}}_1\\
&\text { s.t. } \quad \dualz_{3}=-c\\
&W_{1}^{\top} \dualz_{2}=-\psi\\
&\left[\dualz_{2}\right]_{j}=0, j \in \I_{i}^{-}\\
&\left[\dualz_{2}\right]_{j}=\left[W_{2}^{\top} \dualz_{3}\right]_{j}, j \in \I_{i}^{+}\\
&\left.\begin{array}{ll}
\left(\pub_{j}-\plb_{j}\right) \lambda_{j}-\mu_{j}-\tau_{j} & =\left[W_{2}^{\top} \dualz_{3}\right]_{j} \\
{\left[\dualz_{2}\right]_{j}} & =\pub_{j} \lambda_{j}-\tau_{j}
\end{array}\right\} j \in \I\\
&\lambda, \tau, \mu \geq 0.
\end{aligned}
\end{equation*}
Note that the dual variable $\lambda$ corresponds to the upper bounds in the ReLU relaxation, while $\mu$ and $\tau$ correspond to the lower bounds. By the complementarity property, we know that at the optimal solution, these variables will be zero if the ReLU constraint is non-tight or non-zero if the ReLU constraint is tight.  Since the upper and lower bounds cannot be tight simultaneously, either $\lambda$ or $\mu + \tau$ must be zero. This means that at the optimal solution to the dual problem, we can decompose $[\weight_2^\top\dualz_3]_j$ into positive and negative parts since $(\pub_j-\plb_j)\lambda_j \geq 0$ and $\tau_j + \mu_j \geq 0$ :
\begin{equation*}
\begin{aligned}
	(\pub_j - \plb_j)\lambda_j = [\weight_2^\top \dualz_3]_j^+ \\ \tau_j + \mu_j = [\weight_2^\top \dualz_3]_j^-
\end{aligned}
\end{equation*}
combining this with the constraint $[\dualz_2]_j = \pub_j\lambda_j - \tau_j$ leads to
\begin{equation*}
[\dualz_2]_j = \frac{\pub_j}{\pub_j-\plb_j}[\weight_2^\top \dualz_3]_j^+ - \alpha_j [\weight_2^\top \dualz_3]_j^-,
\end{equation*}
for $j \in \I$ and $ 0 \leq \alpha_j \leq 1$. Hence, we have 
\begin{equation*}
	\lambda_j = \frac{\pub_{ j}}{\pub_j-\plb_j}[\hat{\dualz}_2]_j^+.
\end{equation*}
Now, we denote $\hat{\dualz}_1 = -\psi$ to make our notation consistent, and putting all of this together, the dual objective becomes
\begin{equation*}
\begin{aligned}
-\sum_{i=1}^{2} \dualz_{i+1}^{\top} \bias_{i}+\sum_{j \in \I} \lambda_{ j} \pub_{ j} \plb_{ j}+\psi^{\top} x- \epsilon |\psi_1| = -\sum_{i=1}^{2} \dualz_{i+1}^{\top} \bias_{i}+\sum_{j \in \I} \frac{\pub_{ j} \plb_{ j}}{\pub_j-\plb_j}[\hat{\dualz}_2]_j^+ -\hat{\dualz}_1^{\top} x- \epsilon |[\hat{\dualz}_1]_1| \\= -\sum_{i=1}^{2} \dualz_{i+1}^{\top} \bias_{i}+\sum_{j \in \I}  \plb_{ j}[\dualz_2]_j^+ -\hat{\dualz}_1^{\top} x- \epsilon |[\hat{\dualz}_1]_1|,
\end{aligned}
\end{equation*}
and the final dual problem:
\begin{equation*}
    \begin{array}{ll}
\underset{\dualz, \hat{\dualz}}{\max} & -\sum_{i=1}^{2} \dualz_{i+1}^{\top} \bias_{i}+\sum_{j \in \I} \plb_{ j} [\dualz_2]_j^+-\hat{\dualz}_1^{\top} x- \epsilon |[\hat{\dualz}_1]_1|\\
\text { s.t. } & \dualz_{3}= -c \\
& \hat{\dualz_2} = \weight_2^\top\dualz_3\\
& [\dualz_{2}]_j=0, \;j \in \I^{-} \\
& [\dualz_2]_{ j}=\left[\hat{\dualz}_2\right]_{j}, \;j \in \I^{+} \\
&[\dualz_2]_{j} = \frac{\pub_j}{\pub_j-\plb_j}[\hat{\dualz}_2]_j^+ - \alpha_j[\hat{\dualz}_2]_j^- , \; j \in \I\\
& \hat{\dualz_1} = \weight_1^\top\dualz_2.
\end{array}
\end{equation*}
\end{proof}
Further, we address here the problem of obtaining the upper and lower bounds $\pub$ and $\plb$ for the pre-activations $\hat{\hidden}$. Specifically, the following proposition  gives a closed-form solution.
\begin{lemma}
\label{lemma:bounds}
   Consider the neural network \(\nn\) defined in \Cref{eq:lp_one_layer_net}. Let $w_1$ be the first column of $\weight_1$. Then, for a data point $x$ and perturbation budget \(\epsilon\), we have the following element-wise bounds on the pre-activation vector \(\hat{\hidden}_2\):
    \begin{equation*}
        \plb \leq \hat{\hidden}_2 \leq \pub,
    \end{equation*}
    where
    \begin{equation*}
        \plb = \weight_1x + \bias_1 -\epsilon |w_1|\; \;\text{and} \; \; \pub = \weight_1 x  + \bias_1 +\epsilon |w_1|.
    \end{equation*}
\end{lemma}
	
\begin{proof}
Given a data point $x$ and perturbation budget \(\epsilon\), let $\xpert = x + \delta$ be the perturbed input to the network. First, we find an upper bound to the pre-activations values $\hat{\hidden}_2$:
\begin{equation*}
    \hat{\hidden}_2 = \weight_1(x+\pert) + \bias_1 = \weight_1x + \bias_1 + \weight_1\pert.
\end{equation*}
In particular, we want to solve the following optimisation problem for each component of the pre-activation vector:
\begin{equation*}
\pub_i = \underset{\xpert \in \BB_\epsilon(x) }{\max} [\hat{\hidden}_2]_i = [\weight_1x]_i + [\bias_1]_i + \underset{\xpert \in \BB_\epsilon(x) }{\max} [\weight_1 \pert]_i,
\end{equation*}
where $\pub$ will be the vector containing element-wise upper bounds.
Note that $\pert =  \beta \basis_{1}$, thus the optimisation problem can be rewritten as
\begin{equation*}
\underset{\xpert \in \BB_\epsilon(x) }{\max} [\weight_1 \pert]_i = \underset{|\beta| \leq \epsilon }{\max} \beta \cdot [w_1]_i = \epsilon \cdot |[w_1]_i|,
\end{equation*}
where $w_1 $ is the first column of $W_1$. The vector of the upper bounds will then be:
\begin{equation*}
    u = W_1x + b_1 + \epsilon |w_1|.
\end{equation*}
Along the same lines, we can derive the vector of lower bounds \(\plb\):
\begin{equation*}
    l = W_1x + b_1 - \epsilon |w_1|.
\end{equation*}
\end{proof}

\subsection{Proof of Lemma~\ref{lemma:coapgrad}}
We now consider the dual approximation $\certobj$  to the optimisation problem in~\Cref{eq:adv_maximization}. In what follows, we abuse notation and denote
%Note that, for a binary classification problem, we have \(c=\sgn(y)\) and the dual objective in becomes 
\begin{align}
\certobj\left(x , y\right) = \certobj\left(x , \backnn (\sgn(y),\alpha)\right) ,
\end{align}
where the right hand side is defined in~\Cref{thm:signal_dual_LP} 
where we set \(\alpha\) to the dual feasible solution, and for the sake of clarity, we omit the dependence on the network parameters \(\theta\). 

We are particularly interested in the data points for which $\advobj(x,y) \neq \certobj(x,y)$, i.e. when the certified and adversarial training objectives differ. Below, we provide a necessary and sufficient condition to have a mismatch between the two objectives.

%\coapgrad*

\begin{proof}
For the sake of clarity, we report here the definition of \wong objective from \Cref{thm:signal_dual_LP}. 
\begin{align}
\label{eq:jtilde}
     \certobj(x,y) = -\sum_{i=1}^{2} \dualz_{i+1}^{\top} \bias_{i}+\sum_{j \in \I} \plb_{ j} [\dualz_2]_j^+-\hat{\dualz}_1^{\top} x- \epsilon|[\hat{\dualz}_1]_1|.
\end{align}
Further, recall that the dual variables \( \nu \) are given by the following equations:
\begin{align*}
    \begin{array}{ll}
& \dualz_{3}= -c \\
& \hat{\dualz_2} = \weight_2^\top\dualz_3\\
& [\dualz_{2}]_j=0, \;j \in \I^{-} \\
& [\dualz_2]_{ j}=\left[\hat{\dualz}_2\right]_{j}, \;j \in \I^{+} \\
&[\dualz_2]_{j} = \frac{\pub_j}{\pub_j-\plb_j}[\hat{\dualz}_2]_j^+ - \alpha_j[\hat{\dualz}_2]_j^- , \; j \in \I\\
& \hat{\dualz_1} = \weight_1^\top\dualz_2, \\
\end{array}
\end{align*}
where  $\I^-,\I^+$ and $\I$ denote the sets of activations  in the hidden layer where $\plb$ and $\pub$ are both negative, both positive and span zero, respectively. 


First, we consider the case when the neuron is always dead, i.e., \(\plb < \pub < 0 \). The dual variables are:
\begin{equation*}
    \begin{aligned}
        &\nu_3 = -\sgn(y)\\
& \hat{\nu}_2 =  -a\sgn(y) \\
		&\nu_2 = 0 \\
		&\hat{\nu}_1 =0.
    \end{aligned}
\end{equation*}
Hence, \madry and \wong objectives are equal in this case:
\begin{equation*}
    \certobj = \sgn(y) \bias= \advobj,
\end{equation*}
where the last equality follows from \Cref{eq:exact_j}.


Next, we consider the case when the neuron is always active, i.e., \(\ 0 < \plb < \pub \). The dual variables are:
\begin{equation*}
    \begin{aligned}
        &\nu_3 = -\sgn(y)\\
& \hat{\nu}_2 =  -a\sgn(y) \\
		&\nu_2 = -a\sgn(y)\\
		&\hat{\nu}_1 =-a\sgn(y) \cdot \theta ,
    \end{aligned}
\end{equation*}
and the dual objective becomes
    \begin{align*}
        \certobj &=   - \nu_3^\top \bias - \hat{\nu}_1^\top x - \epsilon | [\hat{\nu}_1]_1 |\\
        &= \sgn(y) \left ( \bias + a( \theta^\top x) \right) - \epsilon |a \sgn(y) \psig | \\
        &= \begin{cases} 
 \sgn(y) \left(\bias + a  \plb \right)& \; \text{if} \; \; a\sgn(y) > 0\\
 \sgn(y) \left(b + a  \pub \right)& \; \text{if} \; \; a\sgn(y) < 0\\
   \end{cases} \\ &= \advobj,
    \end{align*}
where the last equality follows from the fact that $0 < \plb < \pub$. 

 Finally, we consider the case when the neuron is in the activation set $\I$, i.e., $\plb < 0 < \pub$. The dual variables are:
\begin{equation*}
    \begin{aligned}
        &\nu_3 = -\sgn(y) \\
& \hat{\nu}_2 =  -a\sgn(y) \\
		&\nu_2 =  -a\sgn(y) \frac{ \pub}{2\epsilon |\psig}| \\
		&\hat{\nu}_1 =-a\sgn(y)  \frac{ \pub}{2\epsilon |\psig|} \cdot \theta.
    \end{aligned}
\end{equation*}
Here we have two cases, when $\hat{\nu}_2>0$ we can rewrite the dual objective as
\begin{equation*}
    \certobj =  \sgn(y)  \left(\bias  + a \pub \right) = \advobj,
\end{equation*}
and the two objectives coincide. 

When $\nu_2<0$, we can rewrite the dual objective as
\begin{equation*}
\label{eq:cert_obj_on_Istar}
    \certobj = \sgn(y) \left(\bias  + \frac{a \pub \plb}{2\epsilon |\psig|}\right) \neq J_\epsilon.
\end{equation*}
Hence, the only case when \wong gradient differs from \madry gradient is when $\nu_2 < 0$ and the neuron belongs to the activation set $\I$. 

We compute the partial derivative w.r.t. the signal parameter $\psig$ in this case, by the chain rule we have:
\begin{align*}
    &\frac{\partial}{\partial \psig} \loss\left(\sgn(y) \cdot \certobj, y \right) \\&= \frac{\partial}{\partial \certobj} \loss \left(\sgn(y) \cdot \certobj, y\right) \cdot  \frac{\partial}{\partial \psig} \certobj \\&=  \sgn(y)\left[\sigmoid{\sgn(y) \cdot \certobj}- \indicator{ y=1 } \right] \cdot \frac{\partial}{\partial \psig}\certobj
    \\&=  -\frac{a \sgn(y)\sigmoid{ -\certobj }}{2\epsilon}  \left( \frac{\plb}{|\psig|} (\xsig+\epsilon \sgn(\psig)) + \pub \frac{\xsig |\psig|- \theta^\top x \sgn(\psig) }{\psig^2}\right).
\end{align*}
\end{proof}

 

\subsection{Lower bound on the  difference of Gaussian CDFs}

\begin{lemma}
\label{lemma:lb_gausscdfs}
Let \(\gausscdf\) and \(\gausspdf\) be respectively the CDF and PDF of the standard Gaussian distribution. Then, if $x<y<0$ we have
\begin{equation*}
	\phi(0) \left(y-x+\frac{x^3}{6}\right) \leq \gausscdf(y)-\gausscdf(x).
\end{equation*}  
\end{lemma}
 
 \begin{proof}
 	First, we want to prove that $\frac{2x}{\sqrt{\pi}}$ is a   lower bound for the error function $\erf(x)$ when $x \leq 0$. That is, we want to show that $f(x)\geq0$ where $f: (-\infty,0] \to \RR$ is the function defined by
 	\begin{equation*}
 		f(x) = \erf(x) - \frac{2x}{\sqrt{\pi}}.
 	\end{equation*}
 	Since $f$ is continuous and $f(x) \to \infty$ as $x \to -\infty$, $f$ must attain an absolute minimimum on the interval $(-\infty,0]$. Now, differentiating we have
 	\begin{equation*}
 		f^\prime(x) = \frac{2}{\sqrt{\pi}} \exp(-x^2) -\frac{2}{\sqrt{\pi}},
 	\end{equation*} 
 	hence $f$ attains an absolute minimum at $0$ and we have $f(x) \geq f(0) =0$. \newline Next, we show that $\frac{2}{\sqrt{\pi}}(x-x^3/3)$ is an upper bound for $\erf(x)$ when $x \leq 0$. Let $g: (-\infty,0] \to \RR $ the function defined by
 	\begin{equation*}
 		g(x) =  \frac{2}{\sqrt{\pi}}(x-x^3/3)
 		-\erf(x).
 	\end{equation*} 
 	Similarly, since $g$ is continuous and $g(x) \to \infty$ as $x \to -\infty$, $g$ must attain an absolute minimimum on the interval $(-\infty,0]$. Now, differentiating we have
 	\begin{equation*}
 		g^\prime(x) = \frac{2}{\sqrt{\pi}} (1-x^2 -\exp(-x^2)),
 	\end{equation*}
 	hence $g$ attains an absolute minimum at $0$ and we have $g(x) \geq g(0) =0$. \newline Now, since $a < b < 0$ we can use the $\erf$ bounds derived above:
 	\begin{align*}
 		\gausscdf(b)-\gausscdf(a) &= \frac{1}{2} \left( \erf(b/\sqrt{2}) - \erf(a/\sqrt{2}) \right) \\ 
 		&\geq \frac{1}{\sqrt{\pi}} \left( \frac{b}{\sqrt{2}} - \frac{a}{\sqrt{2}} +\frac{a^3}{6\sqrt{2}}\right)\\
 		&=\phi(0) \left(b-a+\frac{a^3}{6}\right),
 	\end{align*}
 	which concludes the proof.
 	 \end{proof}

\subsection{Proof of~\Cref{lemma:negative_bound}}

%\negativebound*

\begin{proof}
	We begin by providing a lower bound on the difference of gaussian cdfs. Applying  \Cref{lemma:lb_gausscdfs}  with $x=\alpha$ and $y=\beta$ we have 	\begin{equation*}
		\gausscdf(\beta) -\gausscdf(\alpha)  \geq \left(\frac{2\epsilon}{r\stdsig} -\frac{(\margin+\epsilon)^3}{6\stdsig^3 r^3}\right)\gausspdf(0), \;\;  \alpha< \beta < 0.
	\end{equation*}
	
Next, we can upper-bound $f$:
\begin{align*}
	f(r) &\leq \margin^2 -\epsilon^2 - 2\stdsig^2 r^2 - \stdsig r \frac{(\margin -3\epsilon)\gausspdf(\beta)  - (\margin+\epsilon)\gausspdf(\alpha) }{\left(\frac{2\epsilon}{\stdsig r} -\frac{(\margin+\epsilon)^3}{6\stdsig^3r^3}\right)\gausspdf(0)}\\
	&\leq \margin^2 -\epsilon^2 - 2\stdsig^2 r^2 - \stdsig^2 r^2 \frac{(\margin -3\epsilon)\gausspdf(0)  - (\margin+\epsilon)\gausspdf(\alpha) }{\left(2\epsilon -\frac{(\margin+\epsilon)^3}{6r^2 \stdsig^2}\right)\gausspdf(0)}
	\\&= \margin^2 -\epsilon^2 - 2\stdsig^2 r^2 - \stdsig^2 r^2 \frac{(\margin -3\epsilon) - (\margin+\epsilon)\exp(-\alpha^2/2) }{2\epsilon -\frac{(\margin+\epsilon)^3}{6\stdsig^2 r^2}}.
	\end{align*}

Now, we use the following upper-bound for the exponential function 
\begin{equation*}
	\exp(x) \leq 1+x-x^2/2, \;\; \forall x \leq 0,
\end{equation*}
and substituting it back into our upper bound for $f$ we get
\begin{equation*}
	f(r) \leq   \margin^2 -\epsilon^2 - 2\stdsig^2 r^2 - \stdsig^2 r^2 \frac{(\margin -3\epsilon) - (\margin+\epsilon)(1- \frac{(\margin+\epsilon)^2}{2r^2\stdsig^2} + \frac{(\margin+\epsilon)^4}{8r^4\stdsig^4}) }{2\epsilon -\frac{(\margin+\epsilon)^3}{6r^2\stdsig^2}},
\end{equation*}

which can be further simplified as
\begin{align*}
		f(r) &\leq   \margin^2 -\epsilon^2 - 2\stdsig^2 r^2 - \stdsig^2 r^2 \frac{(\margin -3\epsilon) - (\margin+\epsilon)(1- \frac{(\margin+\epsilon)^2}{2r^2\stdsig^2} + \frac{(\margin+\epsilon)^4}{8r^4\stdsig^4}) }{2\epsilon -\frac{(\margin+\epsilon)^3}{6r^2\stdsig^2}} \\
		&=\frac{(\margin-7\epsilon)(\margin+\epsilon)^4 + 4r^2\stdsig^2(\margin+\epsilon)(\margin^2-10\margin\epsilon+13\epsilon^2)}{4(\margin+\epsilon)^3 -48r^2\stdsig^2\epsilon} \\&= u(r).
\end{align*}
Hence, we have that for $\epsilon >  \frac{5+2\sqrt{3}}{13} \margin$ and $r> \sqrt{\max\left(\frac{(7\epsilon-\margin)(\margin+\epsilon)^4}{4\stdsig^2(\margin^2-10\margin \epsilon +13\epsilon^2)},\frac{(\margin+\epsilon)^3}{12\stdsig^2\epsilon}  \right)}$ the upper bound is negative, i.e. $u(r) < 0$. %Finally, for the sake of clarity we can further simplify the condition on $r$:
%\begin{equation*}
	%r > \sqrt{\frac{24 \margin^3}{\stdsig^2}} >\sqrt{\max\left(\frac{(7\epsilon-\margin)(\margin+\epsilon)^4}{4\stdsig^2(\margin^2-10\margin \epsilon +13\epsilon^2)},\frac{(\margin+\epsilon)^3}{12\stdsig^2\epsilon}  \right)} 
%\end{equation*}
%which concludes the proof.
\end{proof}
