# Supplementary material for: How robust accuracy suffers from certified training with convex relaxations
Source: arXiv:2306.06995 source file (2023-06-12)
Supplement: Supplementary file 2 [file theory.tex]

In this section, we prove that, for a perfectly aligned threat model, a small margin is sufficient to observe the robust error gap between \wong and \madry. In particular, our result holds for a linearly separable distribution with margin $\gamma$ and a simple neural network.  Below, we
outline our theoretical setting in more detail.



\paragraph{Data and threat model} 
To
sample a data point from the linearly separable distribution with
margin \(\gamma>0\), first we sample the label $y \in \{+1,-1\}$ with
equal probability.  Then, sample $\tilde{x} \in \mathbb{R}^{d-1}$ from
a standard normal distribution  $\xnoise \sim \gauss \left(0,
\stdsig^2 I_{\di-1}\right)$ and set the covariate vector $x = [\margin
\sgn(y);\tilde{x}]$, where  \([;]\) is the concatenation operator. Observe that for the linearly separable distribution, the signal direction
corresponds to the first index of the
input.

We choose our threat model to maximise the alignment with the signal direction.  Hence, we define the set of allowed perturbations
\begin{align}
\label{eq:threat_signal} 
	\BB_\epsilon(x)=\left\{\hidden_1 = x+ \basis_{1} \beta  \mid |\beta|  \leq \epsilon\right\},
\end{align}
where $e_1$ is the canonical basis vector of the first coordinate. Further, we focus on consistent perturbations, i.e. $\epsilon < \gamma$, and we derive an 
extension of the convex outer adversarial
polytope~(\wong)~\citep{wong_provable_2018} for this threat model in~\Cref{apx:certified_training}.


\paragraph{One step gradient descent} We study the early phase of neural network optimisation. Under structural assumptions on the data, it has been proven that one gradient step with sufficiently
large learning rate can drastically decrease the training loss
\cite{chatterji_when_2021} and extract task-relevant features
\cite{frei_random_2022,daniely_learning_2020}.  A similar setting was
also studied recently in \citet{ba_high-dimensional_2022} for the MSE
loss in the high-dimensional asymptotic limit. We focus on 
the classification setting with binary cross-entropy loss:
\begin{align}
\label{eq:loss}
    \loss(x,y) = 
 y \log \left(\sigmoid{x}\right)+\left(1-y\right) \log
 \left(1-\sigmoid{x}\right),
\end{align}
where \(\sigmoid{\cdot}\) is the sigmoid function.
\paragraph{One neuron neural network} Consider the hypothesis class of
one-neuron shallow neural networks $\nn :\RR^{d}\xrightarrow{} \RR$,
\begin{align}
\label{eq:single_neuron_network}
	\nn(x) = a \relu{\theta^\top x} + b ,
\end{align}  
where $x, \theta \in \RR^\di$ and $a,b \in \RR$ and
the only trainable parameter is $\nnparam_1$. Note that as our distribution is linearly separable, our hypothesis class includes the ground truth.

  We are now ready to present our theoretical result for the linearly separable distribution. In particular, \Cref{thm:robustness_gap} shows for a simple neural network that, in high dimensions, certified
training ($\wong$) yield higher robust error than adversarial training ($\madry$) when the margin of the data distribution is small.

\begin{restatable}{theorem}{robustnessgap}
 \label{thm:robustness_gap}
 Let $\rrisk$ be the robust error of $\nn$, defined as 
\begin{align*}
	\rrisk(\theta)  \defn \prob_{(x, y)}\left[\exists z \in \BB_\epsilon(x) : y \neq \sgn\left(\nn(z)\right)\right].
\end{align*}
    Let $\padv$ and $\pcert$ be the network parameters after one step
    of gradient descent with respect to  $\madry$ and $\wong$
    objectives. If the initialised network parameters $\theta$
    satisfy
\begin{align*}
 	\frac{\norm{\pnoise}_2}{\norm{\psig}_2} > \sqrt{\max\left(\frac{(7\epsilon-\margin)(\margin+\epsilon)^4}{4\stdsig^2(\margin^2-10\margin \epsilon +13\epsilon^2)},\frac{(\margin+\epsilon)^3}{12\stdsig^2\epsilon}  \right)},
 \end{align*}
 and \(  \margin < \frac{3}{2}\epsilon \) , $\wong$ yields
        higher robust risk than $\madry$, that is
        \begin{equation*}
        \rrisk(\pcert)> \rrisk(\padv).    
        \end{equation*} 
        %Further,
       % \wong yields higher accuracy discrepancy than \madry:
 %\begin{align*}
% \operatorname{max}_k \mathbf{R}^k(\pcert) - \mathbf{R}(\pcert) > \operatorname{max}_k  \mathbf{R}^k(\padv) - \mathbf{R}(\padv).
% \end{align*}
   
%Further, let:
%\begin{align}
%	\rrisk^k(\theta)  \defn \prob_{(x, y)}\left[\exists z \in \BB_\epsilon(x) : y \neq \sgn\left(\nn(z)\right) \mid y=k\right] 
\end{restatable}
\Cref{thm:robustness_gap} relies on two main assumptions. The first is
an assumption on the data dimensionality and  the initialisation of
the network parameters \(\theta\). For instance, if we initialise the
network parameters \(\theta\) by sampling from a sub-Gaussian
distribution, then the euclidean norm \(\norm{\theta}_2\) concentrates
around \(\sqrt{d}\) with high probability. Hence, the  assumption is
satisfied when the data dimensionality \(d\) is sufficiently high. The
second assumption requires that the implicit margin of the data \(\gamma\)
is sufficiently small, or equivalently that the perturbation budget $\epsilon$ is sufficiently large. This
provides further evidence that a small margin or a large perturbation budget are sufficient to
observe the robust error gap between \wong and \madry. 


\subsection{Proof of~\Cref{thm:robustness_gap}}
We assume, without loss of generality, that at initialisation $\psig >0$, and since $a$ and $b$ are not trainable parameters, we must have $a>0$ and $b<0$ to include the ground truth in our hypothesis class. 

\paragraph{Adversarial training~(\madry)} First of all, note that when \(L\) is the binary cross-entropy loss function, we can rewrite the inner maximisation problem as 
\begin{equation}\label{eq:adv_maximization}
\begin{aligned}
 \underset{x+\delta \in \BB_{\epsilon}(x)}{\operatorname{max}} L(\nn(x + \delta),y)
 = L \left(\sgn(y) \overbrace{\underset{x+\delta \in \BB_{\epsilon}(x)}{\operatorname{min}} \sgn(y) \nn(x+\delta)}^{\defn \advobj(x,y)},\;y \right).
\end{aligned}
\end{equation}
Below, we provide the gradient of the adversarial training objective in Equation \eqref{eq:adv_maximization} w.r.t. the network parameters \(\theta\).

\begin{restatable}{lemma}{advgrad}
\label{lemma:advgrad}
   Consider the neural network \(\nn\) defined in \Cref{eq:single_neuron_network} and the threat model \(\BB_\epsilon\) defined in~\Cref{eq:threat_signal}. Let \(L
   \) be the binary cross-entropy loss function, as defined in \Cref{eq:loss}. Then, we have
\begin{align}
&\nabla_{\theta_1} \max_{x+\delta \in \BB_{\epsilon}(x)} L(\nn(x + \delta),y) \nonumber
 \\ &= -\sgn(y)\sigmoid{-\advobj(x,y)}  \begin{cases} 
a(x_1-\epsilon \sgn(\psig))\indicator{ \plb > 0 }& \; \text{if} \; \; a\sgn(y) > 0 \nonumber\\
 a (x_1+\epsilon \sgn(\psig))\indicator{ \pub> 0 }& \; \text{if} \; \; a\sgn(y) < 0\end{cases} \nonumber,
\end{align}

where $\plb = \theta^\top x - \epsilon |\psig|$ and $\pub = \theta^\top x + \epsilon |\psig|$ are respectively lower and upper bounds on the \(\operatorname{ReLU}\) inputs.
\end{restatable}




%Let $\advobj$ be the adversarial training inner maximisation as defined in~\Cref{eq:adv_maximization}. Then, \madry solves the following optimisation problem:
%\begin{align*}
%	\min_{\theta} \EE_{(x,y)}\left[L\left( \sigmoid{\sgn(y)\advobj(x,y)},y\right)\right]
%\end{align*}
\paragraph{Certified training (\wong)}
Next, we consider the dual approximation $\certobj(x,y)$  to the optimisation problem in~\Cref{eq:adv_maximization}, originally derived in~\citet{wong_provable_2018}. We restate the dual objective $\certobj(x,y)$ in~\Cref{eq:jtilde} and refer the reader to~\Cref{apx:certified_training} for a thorough discussion of certified training dual approximation.

We are particularly interested in the data points for which $\advobj(x,y) \neq \certobj(x,y)$, i.e. when the certified and adversarial training objectives differ. Below, we provide a necessary and sufficient condition to have a mismatch between the two objectives.

\begin{restatable}{lemma}{coapgrad}
\label{lemma:coapgrad}

 Consider the neural network \(\nn\) defined in \Cref{eq:single_neuron_network} and the threat model \(\BB_\epsilon\) defined in~\Cref{eq:threat_signal}. Let \(L
   \) be the binary cross-entropy loss function, as defined in \Cref{eq:loss}. Further, we define $\plb = \theta^\top x - \epsilon |\psig|$ and $\pub = \theta^\top x + \epsilon |\psig|$ respectively as lower and upper bounds on the \(\operatorname{ReLU}\) inputs.
  Let  $\I^\star  = \{(x,y):0 \in [\plb,\pub] \wedge a\sgn(y) > 0\}$. Then, for data points in \(\I^\star\), we have that \madry and \wong gradients differ
\begin{align*}
	\nabla_{\theta_1} \advobj(x,y) \neq \nabla_{\theta_1} \certobj(x,y) \; \; \forall (x,y) \in \I^\star,
\nonumber
\end{align*}
and the \wong gradient is given by
\begin{align}
	&\nabla_{\theta_1} L( \sgn(y)\certobj(x,y), y ) \nonumber\\
	&=   -\frac{a \sgn(y)\sigmoid{ -\certobj(x,y)}}{2\epsilon}  \left( \frac{\plb}{|\psig|} (\xsig+\epsilon \sgn(\psig)) + \pub \frac{\xsig |\psig| - \theta^\top x \sgn( \psig) }{\psig^2}\right) \nonumber.
\end{align}
Further, for data points that are not in \(\I^\star\) we have that \madry and \wong gradients are equivalent
\begin{align}
	\nabla_{\theta_1} \advobj(x,y) = \nabla_{\theta_1} \certobj(x,y) \;\; \forall (x,y) \notin \I^\star \nonumber.
	\end{align}
\end{restatable} 

%Similarly, let $\certobj$ be the COAP dual approximation to the inner maximization described in \Cref{eq:coap_obj}. Then, \wong solves the following optimisation problem:
%\begin{align*}
	%\min_{\theta} \EE_{(x,y)}\left[L\left( \sigmoid{\sgn(y)\certobj},y\right)\right]
%\end{align*}

\paragraph{COAP vs. AT after one step of gradient descent}
Since we are only training the network parameter \(\theta_1\), after one gradient descent step, we have
$\padv_{2:d} = \pcert_{2:d}$.
 Further, we can relate the robust error of the classifier \(\nn\) to the parameter \(\theta_1\) and show that the robust error monotonically decreases in \(\theta_1\), summarized in the following lemma.

\begin{restatable}{lemma}{robustrisk}
\label{lemma:robust_risk}
Let $\nn$ be the neural network defined in \Cref{eq:single_neuron_network} and \(\BB_\epsilon\) the threat model defined in \Cref{eq:threat_signal}. We define the robust error $\rrisk$ of $\nn$ as 
\begin{align*}
	\rrisk(\theta)  \defn \prob_{(x, y)}\left[\exists z \in \BB_\epsilon(x) : y \neq \sgn\left(\nn(z)\right)\right].
\end{align*}
Then, $\rrisk(\theta)$ is monotonically decreasing in $\theta_1$.
\end{restatable}






It follows from~\Cref{lemma:robust_risk} that \madry yields a smaller robust risk than \wong if the following holds:
\begin{equation*}
      \padv_1 > \pcert_1 \implies   \rrisk(\pcert)> \rrisk(\padv).   
\end{equation*}
Further, after one step of gradient descent, the left hand side $\padv > \pcert$ is equivalent to
\begin{align*}
      \EE_{(x,y)}\left[\grad_{\theta_1} L\left( \sigmoid{\sgn(y)\advobj(x,y)} ,y\right)\right] < \EE_{(x,y)} \left[\grad_{\theta_1} L\left( \sigmoid{\sgn(y)\certobj(x,y)} ,y\right) \right] \nonumber.
\end{align*}
Now recall from~\Cref{lemma:advgrad,lemma:coapgrad} that the gradients of \madry and \wong differ only on the set $\I^\star$. In particular, we have that 
\begin{align*}
    (x,y) \notin \I^\star \implies   \grad_{\theta_1} L\left( \sigmoid{\sgn(y)\advobj(x,y)} ,y\right) = \grad_{\theta_1} L\left( \sigmoid{\sgn(y)\certobj(x,y)} ,y\right) < 0 \nonumber,
\end{align*}
and 
\begin{align*}
     (x,y) \in \I^\star \implies  0= \grad_{\theta_1} L\left( \sigmoid{\sgn(y)\advobj(x,y)} ,y\right)  \neq  \grad_{\theta_1} L\left( \sigmoid{\sgn(y)\certobj(x,y)} ,y\right) \nonumber.
\end{align*}
Hence, for our purpose, we need to show that
\begin{align}
\label{eq:exp_grad_Istar}
    \EE_{(x,y)}\left[\grad_{\theta_1} L\left( \sigmoid{\sgn(y)\certobj(x,y)} ,y\right) \mid (x,y) \in \I^\star\right] > 0.
\end{align}

\paragraph{Lower bound on the gradient}
Our strategy will be to lower-bound the expectation in \Cref{eq:exp_grad_Istar} with some strictly positive quantity. We define 
\begin{align*}
	Z = \sum_{i=2}^\di \theta_i x_i
\end{align*}
and plug-in the gradient computed in \Cref{lemma:coapgrad} to obtain

\begin{align*}
    &\EE_{(x,y)} \biggl[ \grad_{\psig}\loss\biggl( \sgn(y)\sigmoid{\certobj(x,y)} ,y\biggr) \bigg| (x,y) \in \I^\star \biggr] \\
    &= \EE_{(x,y)} \biggl[ \frac{a \sigmoid{ - \certobj(x,y)}}{2\epsilon} \biggl( -\frac{\plb}{\psig} (\margin+\epsilon) +\pub \frac{\sum_{i=2}^\di x_i \theta_i}{\psig^2} \biggr) \bigg| (x,y) \in \I^\star \biggr] \nonumber \\
    &= \frac{a}{2 \psig \epsilon} \EE_{(x,y)} \biggl[ \sigmoid{- \certobj(x,y)}\biggl( -\plb (\margin+\epsilon) +\pub \frac{Z}{\psig} \biggr) \bigg| (x,y) \in \I^\star \biggr] \nonumber\\
    &= \frac{a}{2 \psig \epsilon}\EE_{(x,y)} \biggl[  \sigmoid{ - \certobj(x,y)} \pub \frac{Z}{\psig} -  \sigmoid{- \certobj(x,y)}\plb(\margin+\epsilon)  \bigg| (x,y) \in \I^\star \biggr] \nonumber.
\end{align*}
Now, we observe that $Z$ is always negative on the set $\I^\star$, since we need to satisfy the constraint $\plb < 0 <\pub$ we have
\begin{align*}
	(x,y) \in \I^\star \implies -\psig (\margin+\epsilon)  < \sum_{i=2}^\di \theta_i x_i < -\psig (\margin-\epsilon) < 0.
\end{align*}
Further, 
\begin{align*}
 (x,y) \in \I^\star \implies \sigmoid{ -\certobj(x,y)}\geq \frac{1}{2}.
\end{align*}
Combining these two observations, we can lower-bound the expectation 
\begin{align*}
        &\EE_{(x,y)} \left [ \grad_{\psig}\loss\left( \sgn(y)\sigmoid{\certobj(x,y)} ,y\right) \mid  (x,y) \in \I^\star \right]         \\ 
        &= \frac{a}{2 \psig \epsilon}\EE_{(x,y)} \left [ \sigmoid{ - \certobj(x,y)} \pub \frac{Z}{\psig}  - \sigmoid{- \certobj(x,y)}\plb(\margin+\epsilon)   \mid  (x,y) \in \I^\star \right] \nonumber\\
        &\geq \frac{a}{2 \psig \epsilon}\EE_{(x,y)} \left [  \pub \frac{Z}{\psig} -  \frac{\margin+\epsilon}{2}\plb  \mid  (x,y) \in \I^\star \right] \nonumber.
\end{align*}
Now, we need to show that this lower-bound is strictly positive, i.e.
\begin{equation*}
     \EE_{(x,y)} \left [   u \frac{Z}{\psig} - \frac{\margin+\epsilon}{2}\plb   \mid  (x,y) \in \I^\star \right] > 0.
\end{equation*}
Note that we can further expand this expression as
\begin{align*}
   &\EE_{(x,y)} \left [    u \frac{Z}{\psig}  - \frac{\margin+\epsilon}{2}\plb \mid  (x,y) \in \I^\star \right]  \\ 
   &= -(\margin^2 -\epsilon^2)\psig^2 + (\margin+\epsilon)\psig \EE\left[Z \mid  (x,y) \in \I^\star\right] + 2\EE\left[Z^2 \mid  (x,y) \in \I^\star\right] \nonumber.
\end{align*}
Further, $Z \mid   (x,y) \in \I^\star $ is distributed as a truncated normal with
\begin{align*}
	\alpha = -\frac{\psig(\margin+\epsilon)}{\stdsig \norm{\pnoise}_2} \; \; \text{and} \; \;\beta = -\frac{\psig(\margin-\epsilon)}{\stdsig \norm{\pnoise}_2}.
\end{align*}  Hence, we can plug in the expectations of the truncated normal distribution to obtain 
\begin{align*}
      &-(\margin^2 -\epsilon^2)\psig^2 + \psig(\margin+\epsilon) \EE\left[Z \mid  (x,y) \in \I^\star\right] +2\EE\left[Z^2 \mid  (x,y) \in \I^\star\right] \nonumber \\  &=
-(\margin^2 -\epsilon^2)\psig^2 + 2\stdsig^2 \norm{\pnoise}_2^2 + \stdsig \norm{\pnoise}_2\psig \frac{(\margin -3\epsilon)\gausspdf(\beta)  - (\margin+\epsilon)\gausspdf(\alpha) }{\gausscdf(\beta)-\gausscdf(\alpha)} \nonumber \\
&\propto -(\margin^2 -\epsilon^2) + 2\stdsig^2 r^2 + \stdsig r \frac{(\margin -3\epsilon)\gausspdf(\beta)  - (\margin+\epsilon)\gausspdf(\alpha) }{\gausscdf(\beta)-\gausscdf(\alpha)} \nonumber \\
&= -f(r),
\end{align*}
where we define $r = \frac{\norm{\pnoise}_2}{|\psig|}$. 

Now, under our assumptions, the following lemma holds.

\begin{restatable}{lemma}{negativebound}
\label{lemma:negative_bound}
    Suppose $f: \RR \to \RR$ is defined as
    \begin{align*}
        f(r) = \margin^2 -\epsilon^2 - 2\stdsig^2 r^2 - \stdsig r \frac{(\margin -3\epsilon)\gausspdf(\beta)  - (\margin+\epsilon)\gausspdf(\alpha) }{\gausscdf(\beta)-\gausscdf(\alpha)},
    \end{align*}
where $\alpha \defn -\frac{\margin+\epsilon}{r\stdsig} $ , $\beta \defn -\frac{\margin-\epsilon}{r\stdsig} $, $\gausscdf$  and $\gausspdf$  are respectively the standard Gaussian CDF and PDF.
 Assume that
\begin{equation*}
	 \frac{5+2\sqrt{3}}{13} \margin < \epsilon < \margin.
\end{equation*}
Then, we have
\begin{align*}
f(r) < 0,\; \; \forall r> \sqrt{\max\left(\frac{(7\epsilon-\margin)(\margin+\epsilon)^4}{4\stdsig^2(\margin^2-10\margin \epsilon +13\epsilon^2)},\frac{(\margin+\epsilon)^3}{12\stdsig^2\epsilon}  \right)}.\end{align*}
\end{restatable}
Hence, it follows that \(\rrisk(\pcert) > \rrisk(\padv)\), which concludes the proof.
